# Supplementary material for: Neural Quasiprobabilistic Likelihood Ratio Estimation with Negatively Weighted Data
Source: arXiv:2410.10216 source file (2024-10-14)
Supplement: Supplementary file 1 [file Appendix_SupervisedLearningPrimer.tex]

{\color{red}REMOVE THIS SECTION?}
The goal of a supervised classification algorithm is to learn a function $s: \mathcal{X} \rightarrow \mathbb{R}$ that maps the input space $\mathcal{X}$ to the supervisory label space $\mathcal{Y}$. This is quantified by the so-called \textit{loss function}, which is a measure of \textit{closeness} between $s(\mathbf{x})$ and $y$ for each realisation, which for the entire dataset is known as the \textit{empirical risk} which in the case of weighted data is: 
\begin{align}
    \label{eq:empirical_loss}
    \mathcal{L}(s) &= \mathbb{E}_{\tilde{X},Y}[w(\tilde{X},Y) \cdot \mathcal{L}(s(\tilde{X}), Y)] \\
    &\approx \frac{1}{N} \cdot \sum^{N}_{i} w_{i} \cdot \mathcal{L}(s(\mathbf{x}_{i}), y_{i})
\end{align} 
%-----------------------
% MATT LEFT OFF EDITING HERE - need to introduce weights as a random variable around this point potentially and condense with Sec 2
%-----------------------

Generally speaking, this learning objective is made tractable by expressing $s(\mathbf{x})$ as a set of $k$ configurable \textit{model} parameters $\theta \in \RealSpace{k}$ ($s(\mathbf{x}) \mapsto s(\mathbf{x};\theta)$). By minimising the loss over the entire dataset, one can configure the function parameters so that  $s(\mathbf{x};\mathbf{\theta})$ most accurately reflects the supervisory labels of the data. The exact form of the learned function can vary wildly, however the adopted method used in this work (due to their differentiable behaviour) are neural networks. With this in mind, the optimisation problem is typically solved using gradient descent algorithms that update the function parameters according to:
\begin{align}
\label{eq:gradient_update}
    \theta^{t+1} = \theta^{t}-\gamma\nabla_{\theta^{t}}\mathcal{L}(s),
\end{align}
where $t$ is an iterative update step, and $\gamma$ is a learning rate \cite{38136}. From a practical perspective \textit{mini-batch} training is often employed, meaning that for a mini-batch of finite size $N_{\textrm{batch}} < N$, the gradient takes the form:
\begin{align}
\label{eq:LossGradient}
\nabla_{\theta^{t}}\mathcal{L}(s) &= \nabla_{\theta^{t}} ( \sum^{N_{\textrm{batch}}}_{i} w_{i} \cdot \mathcal{L}(s(\mathbf{x}_{i};\mathbf{\theta}), y_{i}) ) \notag \\
  &= \sum^{N_{\textrm{batch}}}_{i} w_{i} \cdot \nabla_{\theta^{t}} \mathcal{L}(s(\mathbf{x}_{i};\mathbf{\theta}), y_{i}).
\end{align}
which demonstrates the linear property of the gradient with respect to the sum of each loss term.
